# Supplementary material for: Smoothed Analysis of the k-Swap Neighborhood for Makespan Scheduling
Source: arXiv:2411.17245 source file (2024-11-26)
Supplement: Supplementary file 1 [file Appendix.tex]

\begin{appendices}
\section{Appendix}

\textbf{Proof of Lemma~\ref{lem:graterThanZeroInequality}:} We have the following cases:
    \begin{itemize}
      \item Case 1: In the first case, we have $a > b \geq 0$. Moreover, since $c < a - b$ and $b \geq 0$, we have $c < a$. Therefore, 
      \begin{align*}
            |a - c| + |b + c| = a - c + b + c = a + b = |a| + |b|.
        \end{align*}
      
      \item Case 2: In the second case, we have $b < a < 0$. Moreover, since $b+c < a$, and $a<0$, we have $b+c < 0$. Therefore,
      \begin{align*}
            |a - c| + |b + c| = c - a - b - c = -a - b = |a| + |b|.
        \end{align*}
      
      \item Case 3: In the third case, we have $a \geq 0$ and $b < 0$. For this case, we consider the following subcases:
        \begin{itemize}
            \item Subcase 3.1: If we have $c \geq a$ and $b + c < 0$, we get
            \begin{align*}
            |a - c| + |b + c| = c - a - b - c = -a - b < |a| + |b|.
            \end{align*}
            \item  Subcase 3.2: If we have $c \geq a$ and $b + c \geq 0$, we get
            \begin{align*}
            |a - c| + |b + c| = c - a + b + c < 2a - 2b - a + b = a - b = |a| + |b|.
            \end{align*}
            \item  Subcase 3.3: If we have $c < a$ and $b + c < 0$, we get
            \begin{align*}
            |a - c| + |b + c| = a - c - b - c = a - b -2c < a - b = |a| + |b|.
            \end{align*}
            \item  Subcase 3.4: If we have $c < a$ and $b + c \geq 0$, we get
            \begin{align*}
            |a - c| + |b + c| = a - c + b + c = a + b < |a| + |b|.
            \end{align*}
        \end{itemize}
    \end{itemize}
